# Supplementary material for: AutoWebGLM: A Large Language Model-based Web Navigating Agent
Source: arXiv:2404.03648 source file (2024-10-12)
Supplement: Supplementary file 1 [file demonstration.tex]

\section{Demonstration}\label{app:demo}

\subsection{Weather Report}
The targeted task to be executed is "What is the weather like today?". 
The actual execution steps can be summarized as follows:
\begin{itemize}
    \item Step1: Type SearchBar "todays weather report"
    \item Step2: Click SearchButton
    \item Step3: Click SearchBar
    \item Step4: Click DateButton
    \item Step5: Answer
\end{itemize}
As Figure~\ref{fig:demo1} shows, we end up on the webpage with a local weather report. We obtained detailed information about today's weather as the answer, effectively completing the target task.

\subsection{Shopping Advice}
The targeted task to be executed is "Help me pick a Christmas gift for kids". 
The actual execution steps can be summarized as follows:
\begin{itemize}
    \item Step1: Type SearchBar "Christmas gift for kids"
    \item Step2: Click SearchButton
    \item Step3: Click "All" tag in the category selection
    \item Step4: Click SearchBar
    \item Step5: Click The first product on the result page
    \item Step6: Answer
\end{itemize}
As Figure~\ref{fig:demo2} shows, we ultimately landed on a camera product page, where we obtained a recommendation for that camera as the answer, essentially completing the task.

\subsection{Searching Article}
The targeted task to be executed is "Find an article about large language model". 
The actual execution steps can be summarized as follows:
\begin{itemize}
    \item Step1: Type SearchBar "large language model"
    \item Step2: Click SearchButton
    \item Step3: Click Wiki
    \item Step4: Scroll down
    \item Step5: Go backward
    \item Step6: Scroll down
    \item Step7: Click The link to an article
    \item Step8: Answer
\end{itemize}
As Figure~\ref{fig:demo3} shows, we ultimately arrived at a page featuring an article and obtained "Found a relevant article" as the answer, essentially fulfilling the task.

\subsection{Searching Tools}
The targeted task to be executed is "Find a tool to solve the differential equation". 
The actual execution steps can be summarized as follows:
\begin{itemize}
    \item Step1: Type SearchBar "tools to solve the differential equation"
    \item Step2: Click SearchButton
    \item Step3: Scroll down
    \item Step4: Click The link to an online tool
    \item Step5: Click ODE calculator
    \item Step6: Answer
\end{itemize}
As Figure~\ref{fig:demo4} shows, we ultimately arrived at a page for an ODE (Ordinary Differential Equation) calculator and obtained "Found a relevant tool" as the answer, essentially completing the task.

\subsection{Knowledge Query}
The targeted task to be executed is "Search and tell me some basic info about the dark matter". 
The actual execution steps can be summarized as follows:
\begin{itemize}
    \item Step1: Type SearchBar "dark matter"
    \item Step2: Click SearchButton
    \item Step3: Click Wiki
    \item Step4: Scroll down
    \item Step5: Answer
\end{itemize}
As Figure~\ref{fig:demo6} shows, we ultimately reached a wiki page about dark matter, obtaining some basic info as the answer, and effectively completing the task.

\subsection{Finding Pictures}
The targeted task to be executed is "Help find a beautiful picture of the Pacific Ocean". 
The actual execution steps can be summarized as follows:
\begin{itemize}
    \item Step1: Type SearchBar "Pacific Ocean Pictures"
    \item Step2: Click SearchButton
    \item Step3: Click A picture in the search result
    \item Step4: Go backward
    \item Step5: Click Another in the search result
    \item Step6: Answer
\end{itemize}
As Figure~\ref{fig:demo7} shows, we ultimately reached a page displaying an image of the Pacific Ocean, obtaining "Found a picture of the Pacific Ocean for you" as the answer, effectively completing the task.

\subsection{Finding Research}
The targeted task to be executed is "Search and tell me a hot area in AI research". 
The actual execution steps can be summarized as follows:
\begin{itemize}
    \item Step1: Type SearchBar "areas in AI research"
    \item Step2: Click SearchButton
    \item Step3: Click A Link to a page
    \item Step4: Scroll down
    \item Step5: Answer
\end{itemize}
As Figure~\ref{fig:demo9} shows, we ultimately reached a page about AI research, obtaining "Natural Language Processing(NLP)" as the answer, effectively completing the task.

\subsection{Game Recommendation}
The targeted task to be executed is "I want to play a PC game. Help me choose one". 
The actual execution steps can be summarized as follows:
\begin{itemize}
    \item Step1: Type SearchBar "PC game recommendations"
    \item Step2: Click SearchButton
    \item Step3: Answer
\end{itemize}
As Figure~\ref{fig:demo10} shows, we ultimately reached a page of searching results of games, obtaining a recommendation as the answer, effectively completing the task.

\subsection{Playing Video}
The targeted task to be executed is "Search and tell me a hot area in AI research". 
The actual execution steps can be summarized as follows:
\begin{itemize}
    \item Step1: Type SearchBar "funny videos"
    \item Step2: Click SearchButton
    \item Step3: Click A Link to a vedio
    \item Step4: Answer
\end{itemize}
As Figure~\ref{fig:demo5} shows, we ultimately reached a page playing a funny video, effectively completing the task.

\subsection{Online Shopping Assistance with Pop-Up Interruption}
The targeted task to be executed is "Find and select a highly rated toaster". The actual execution steps can be summarized as follows:
\begin{itemize}
\item Step1: Type SearchBar "best toaster 2024"
\item Step2: Click SearchButton
\item Step3: Click a link from the search results leading to an online shopping site (Encounter a pop-up asking to subscribe to the newsletter.)
\item Step4: Scroll down, but the interaction is blocked by the pop-up
\item Step5: Answer
\end{itemize}
As Figure~\ref{fig:demo14} shows, we do not reach the intended product selection. The presence of an unexpected pop-up interrupts the task execution, demonstrating the system's limitation in handling unexpected graphical elements and pop-ups. This outcome underscores the need for enhanced capabilities in graphical recognition and interaction handling, ensuring smoother navigation and task completion on web pages with complex elements.

\subsection{Knowledge Query with Hallucination}
The targeted task to be executed is "Tell me some basic info about NLP". 
The actual execution steps can be summarized as follows:
\begin{itemize}
    \item Step1: Answer
\end{itemize}
As Figure~\ref{fig:demo12} shows, this case is a classic example of the hallucination fallacy, where the system responded directly without going through the webpage, and the response came from the hallucination rather than the webpage information

\subsection{Technological Breakthrough Summary with misinterpretation}
The targeted task to be executed is "Summarize a recent technological breakthrough in renewable energy". The actual execution steps can be summarized as follows:
\begin{itemize}
\item Step1: Type SearchBar "latest technological breakthrough in renewable energy 2024"
\item Step2: Click SearchButton
\item Step3: Click a link in search results (The system selects a link to a general overview of renewable energy technologies instead of a specific article on recent breakthroughs.)
\item Step4: Scroll down
\item Step5: Answer
\end{itemize}
As Figure~\ref{fig:demo13} shows, we do not reach the intended outcome. Instead of summarizing a recent technological breakthrough, the system provides a generalized overview of renewable energy. This outcome highlights a misinterpretation of task context, demonstrating the system's challenge in distinguishing between general information and specific, recent developments.

\subsection{Map Query with Poor Graphical Recognition}
The targeted task to be executed is "Where is Beijing relative to Shanghai according to the map". 
The actual execution steps can be summarized as follows:
\begin{itemize}
    \item Step1: Type SearchBar "Beijing"
    \item Step2: Click SearchButton
    \item Step3: Answer
\end{itemize}
As Figure~\ref{fig:demo8} shows, we ultimately reached a page displaying a description of Beijing and the Beijing map, obtaining "Northside" as the answer. The answer is to some extent too simple. This case illustrates two minor flaws in our system: one is that it has a slight lack of understanding of the graphical interface, and the other is that it sometimes hallucinates, and the answers it gets are not always from web information. 

\begin{figure*}[htbp]
    \centering
    \includegraphics[width=0.95\linewidth]{images/demo1/2f388f72e54ae7343146fd477612cb5.png}
    \caption{Weather Report}
    \label{fig:demo1}
\end{figure*}

\begin{figure*}[htbp]
    \centering
    \includegraphics[width=0.95\linewidth]{images/demo2/baa9aeeb569c8f7396c41b4956f0348.png}
    \caption{Shopping Advice}
    \label{fig:demo2}
\end{figure*}

\begin{figure*}[htbp]
    \centering
    \includegraphics[width=0.95\linewidth]{images/demo3/a9ff129fdc6cfe0f06c13b012b1dd4c.png}
    \caption{Searching Article}
    \label{fig:demo3}
\end{figure*}

\begin{figure*}[htbp]
    \centering
    \includegraphics[width=0.95\linewidth]{images/demo4/8775a25f268b70ad49081347ba55bc2.png}
    \caption{Searching tools}
    \label{fig:demo4}
\end{figure*}

\begin{figure*}[htbp]
    \centering
    \includegraphics[width=0.95\linewidth]{images/demo6/f570c2fdc633cbd2648a71132df6766.png}
    \caption{Knowledge Query}
    \label{fig:demo6}
\end{figure*}

\begin{figure*}[htbp]
    \centering
    \includegraphics[width=0.95\linewidth]{images/demo7/77809153052743428a03c29a54ceb11.png}
    \caption{Finding Pictures}
    \label{fig:demo7}
\end{figure*}

\begin{figure*}[htbp]
    \centering
    \includegraphics[width=0.95\linewidth]{images/demo9/30b49b57c6fc7b41b5eb785fc1dbf86.png}
    \caption{Finding Research}
    \label{fig:demo9}
\end{figure*}

\begin{figure*}[htbp]
    \centering
    \includegraphics[width=0.95\linewidth]{images/demo10/eef7fea4421344f797386c2dcf5c58c.png}
    \caption{Game Recommendation}
    \label{fig:demo10}
\end{figure*}

\begin{figure*}[htbp]
    \centering
    \includegraphics[width=0.95\linewidth]{images/demo5/b1ac295dd1fc104842cdd4f885b5b78.png}
    \caption{Playing Video}
    \label{fig:demo5}
\end{figure*}

\begin{figure*}[htbp]
\centering
\includegraphics[width=0.95\linewidth]{images/demo14/d15927e46176900141e96136ba70994.png}
\caption{Online Shopping Assistance with Pop-Up Interruption}
\label{fig:demo14}
\end{figure*}

\begin{figure*}[htbp]
    \centering
    \includegraphics[width=0.95\linewidth]{images/demo12/2a7669cc0a7f61ff5101139c752c9af.png}
    \caption{Knowledge Query with Hallucination}
    \label{fig:demo12}
\end{figure*}

\begin{figure*}[htbp]
\centering
\includegraphics[width=0.95\linewidth]{images/demo13/1b53a87e57208a78e4e6756a797fce6.png}
\caption{Technological Breakthrough Summary with misinterpretation}
\label{fig:demo13}
\end{figure*}

\begin{figure*}[htbp]
    \centering
    \includegraphics[width=0.95\linewidth]{images/demo8/2704f4743ad100718915152964a0996.png}
    \caption{Map Query with Poor Graphical Recognition}
    \label{fig:demo8}
\end{figure*}
